# Supplementary material for: Reduced order modeling with time-dependent bases for PDEs with stochastic boundary conditions
Source: arXiv:2112.14326 source file (2022-11-07)
Supplement: Supplementary file 1 [file AppendixA.tex]

The proof of Theorem(\ref{VarTheorem}) is given in detail in Appendix A of \cite{ramezanian2021onthefly}. 
The major differences between the proof given in \cite{ramezanian2021onthefly} and the proof for the equations given in Theorem(\ref{VarTheorem}) are: 
\begin{enumerate}
    \item In this paper, we consider the spatial modes in the discrete sense, whereas they are considered to be continuous in \cite{ramezanian2021onthefly}. The analogous discrete representation of the continuous form, especially the inner products, have been discussed in section \ref{sec:Method}. It has already been established that the discrete representation converges to the continuous form as the number of discrete points are increased. 
    \item The $\bm{y}(t)$-modes in this paper are taken to be modes in the stochastic space whereas they were considered to be orthonormal species modes in \cite{ramezanian2021onthefly}. Therein all the species were considered to be equally weighted. The inner product as given in \cite{ramezanian2021onthefly} is,
    \begin{equation*}
        \bm{y}_i^T \bm{y}_j = \delta_{ij}.
    \end{equation*}
    Whereas, in the stochastic space the samples are weighted. Thus, inner product in the stochastic space also includes the weights of the samples,
    \begin{equation*}
        \bm{y}_i^T \bm{W}_{\xi} \bm{y}_j = \delta_{ij}.
    \end{equation*}
%     \item On taking the time derivative of the orthonormality constraint we obtain the dynamic orthogonality of the modes given by,  
% \begin{align*}
%   \inner{{\mathbf{u}}_{\ol{\mathbf{x}}_i}(t)}{\dot{\mathbf{u}}_{\ol{\mathbf{x}}_j}(t)}_{{{x}}} &= {\varphi}_{ij}(t),\\
%   \inner{\bm{y}_i^T(t)}{\dot{\bm{y}}_j(t)}_{{\xi}} &= \theta_{ij}(t),
% \end{align*}
% where $\boldsymbol{\varphi}(t) \equiv \varphi_{ij}(t)$ and ${\boldsymbol{\theta}}(t) \equiv \theta_{ij}(t)$ are skew-symmetric matrices i.e., $\varphi_{ij}=-\varphi_{ji}$ and $\theta{ij}=-\theta{ji}$.
\end{enumerate}
Taking care of the above mentioned differences in the notation, the proof in \cite{ramezanian2021onthefly} can be easily adapted to the evolution equations in Theorem(\ref{VarTheorem}).    
